# Supplementary material for: An Infrastructure-less, Control-Independent Solution to Relative Localisation of a Team of Mobile Robots using Ranging Measurements
Source: arXiv:2606.20365 source file (2026-06-18)
Supplement: Supplementary file 1 [file 7_appendix.tex]

\subsection{Clustering of Particles} \label{apx:cluster}

After only a few informative measurements, the particle distribution naturally forms coherent spatial clusters. Within each cluster, however, particles may still exhibit distinct orientation modes.

To capture both spatial and heading variability, maximum-entropy distributions suited to each domain are adopted. Spatial positions are modeled with a bivariate Gaussian distribution, while orientations are modeled with the von Mises distribution \cite{vonmises}, which accounts for the periodic nature of angles. The probability density of the von Mises distribution is given by
\begin{equation*}
    \text{VM}(\theta \mid \mu, \kappa) = \frac{1}{2\pi I_0(\kappa)} \exp\left(\kappa \cos(\theta - \mu) \right)
\end{equation*}
where $\mu$ is the mean direction, $\kappa$ is the concentration parameter, and $I_0$ denotes the modified Bessel function of order zero.
The distribution reduces to a uniform density as $\kappa \to 0$, while larger $\kappa$ indicate stronger concentration around $\mu$.
For small dispersions the approximation between variance and concentration factor $\kappa \approx 1/\sigma^2$ holds.

\subsubsection{Gaussian--von Mises Mixture Model (GVMMM)} 
Particles are clustered using a hybrid mixture model that combines Gaussian and von Mises likelihoods. For $K$ candidate clusters, the likelihood of particle $i$ under cluster $k$ is given by
\begin{equation*}
    \mathcal{L}_{ik} = \mathcal{N}\!\left(\mathbf{x}_i \mid \boldsymbol{\mu}_k, \boldsymbol{\Sigma}_k\right)
    \cdot \text{VM}(\theta_i \mid \mu_k^\theta, \kappa_k)
\end{equation*}
where $\mathbf{x}_i$ is the spatial component of the particle, $\theta_i$ its orientation, $(\boldsymbol{\mu}_k,\boldsymbol{\Sigma}_k)$ the Gaussian parameters, and $(\mu_k^\theta, \kappa_k)$ the von Mises parameters.

\noindent Cluster assignment is performed via the Expectation--Maximization (EM) algorithm:
\begin{itemize}
    \item \textbf{E-step:} compute soft responsibilities
    \begin{equation}
        r_{ik} = \frac{w_k \mathcal{L}_{ik}}{\sum_{j=1}^K w_j \mathcal{L}_{ij}}
        \label{eq:resp}
    \end{equation}
    where $w_k$ are cluster weights.
    \item \textbf{M-step:} update parameters using responsibility-weighted statistics.
\end{itemize}

\noindent The Gaussian mean and covariance are updated as
\begin{align*}
    \boldsymbol{\mu}_k &= \frac{\sum_i r_{ik}\mathbf{x}_i}{N_k} \\
    \boldsymbol{\Sigma}_k &= \frac{\sum_i r_{ik}(\mathbf{x}_i-\boldsymbol{\mu}_k)(\mathbf{x}_i-\boldsymbol{\mu}_k)^\top}{N_k}
\end{align*}
where $N_k = \sum_i r_{ik}$
For orientations, the resultant vector
\begin{equation*}
    C_k = \sum_i r_{ik}\cos\theta_i, \quad
    S_k = \sum_i r_{ik}\sin\theta_i 
\end{equation*}
is used to update the mean angle $\mu_k^\theta = \text{atan2}(S_k,C_k)$. 
The concentration parameter $\kappa_k$ is estimated using a truncated Newton method following the approximation scheme described in~\cite{sra2012short}.

\subsubsection{Model Selection}
The number of clusters $K$ is selected using the Bayesian Information Criterion (BIC)
\begin{equation*}
    \mathrm{BIC}(K) = -2 \log \mathcal{L} + \lambda \, p(K) \log n_\text{P}
\end{equation*}
where $\log \mathcal{L}$ is the log-likelihood, $n_\text{P}$ is the number of particles, $p(K)$ the number of free parameters in the model, and $\lambda$ a tunable penalization factor. The clustering is performed for progressively increasing values of $K$ ($K=1,\dots,n_c^{\max}$), and the model yielding the minimal BIC is selected.

\subsubsection{Cluster Representation}
Each particle is assigned to the cluster for which it has the highest posterior responsibility.
Each cluster $c$ is summarized by the descriptor
\[
    \left(\mathbf{q}^{cj,i}, \mathbf{P}^{cj,i}, w^{cj,i}, \kappa^{cj,i}\right)
\]
where $\mathbf{q}^{cj,i}$ is the cluster mean, $\mathbf{P}^{cj,i}$ the covariance, $w^{cj,i}$ the relative weight (fraction of particles), and $\kappa^{cj,i}$ the orientation concentration. These descriptors compactly represent particle hypotheses, facilitating their use in subsequent stages of the algorithm and their exchange among agents.

\subsection{Computation of cluster descriptors}
\label{apx:desc_clust}

When clusters are propagated, their descriptors (mean pose, covariance and dispersion factor) are recomputed from the propagated particles. 
The position $(x,y)$ components are modeled with a Gaussian distribution, while the orientation $\theta$ is modeled with a von Mises distribution. 
Given a set of $n_\text{P}$ propagated particles $\mathbf{q}^{p} = \begin{bmatrix} x^p & y^p & z^p \end{bmatrix}^\top \ \forall p = 1,..,n_\text{P}$
the updated descriptors are obtained as follows:

\begin{enumerate}
    \item \textbf{Position parameters:}
    \begin{align*}
        \mu_{xy} &= \frac{1}{n_\text{P}}\sum_{p=1}^{n_\text{P}}
        \begin{bmatrix}
        x^{pa} \\ y^{pa}
        \end{bmatrix} \\
        \mathbf{P}_{xy} &= \frac{1}{n_\text{P}-1}\sum_{p=1}^{n_\text{P}}
        \bigl(\mathbf{x}^{pa} - \mu_{xy}\bigr)\bigl(\mathbf{x}^{pa} - \mu_{xy}\bigr)^\top
    \end{align*}

    \item \textbf{Heading parameters:}  
    The sum of cartesian contribution is computed as
    \[
        C = \sum_{p=1}^{n_\text{P}} \cos(\theta^{pa}),
        \quad 
        S = \sum_{p=1}^{n_\text{P}} \sin(\theta^{pa})
    \]
    in order to compute the mean of headings
    \[
        \mu_\theta = \operatorname{atan2}(S,C)
    \]
    The concentration parameter $\kappa$ of the von Mises distribution is estimated iteratively from the resultant length
    \[
        R = \frac{\sqrt{C^2+S^2}}{n_\text{P}}
    \]
    Following \cite{sra2012short}, the approximation 
    $\kappa \approx R\frac{2-R^2}{1-R^2}$ 
    is refined via a few Newton iterations.\\
    The heading variance is computed using the circular residuals
    \begin{equation*}
        \sigma^2_\theta = \frac{1}{n_\text{P}-1}\sum_{p=1}^{n_\text{P}}
        \left(\text{mod}(\theta^{pa} - \mu_\theta + \pi, 2\pi) - \pi \right)^2
    \end{equation*}

    \item \textbf{Final cluster descriptor:}  
    The cluster mean and covariance are thus
    \[
        \mu = 
        \begin{bmatrix}
        \mu_{xy} \\ \mu_\theta
        \end{bmatrix}, 
        \quad
        \mathbf{P} = 
        \begin{bmatrix}
        \mathbf{P}_{xy} & 0 \\
        0 & \sigma^2_\theta
        \end{bmatrix}
    \]
\end{enumerate}
